# Supplementary material for: Improving Outbreak Detection with Stacking of Statistical Surveillance Methods
Source: arXiv:1907.07464 source file (2019-07-17)
Supplement: Supplementary file 1 [file appendix.tex]

\begin{table*}
\caption{Results for  the average rank for including the average in the dataset.}
\label{tab:average}
\scriptsize
%\resizebox{\textwidth}{!}{%)
\begin{tabular}{|l|r|r|r|r|r|r|r|}
\hline
approach & overall & $\{\bar T, \bar{S1}, \bar{S2}\}$ &  $\{\bar{T}, S1, \bar{S2}\}$ & $\{\bar{T}, S1, S2\}$ &  $\{ T, \bar{S1}, \bar{S2}\}$ & $\{ T, S1, \bar{S2}\}$ & $\{ T, S1, S2\}$ \\
\hline
\hline
S($\bar \mu$, $O_0$, $0$)  &               3.429 &   3.714 & 3.571 & 3.000 & 3.429 & 3.286 &  3.571 \\
S($ \mu$, $O_0$, $0$)  &               \textbf{3.357} &   2.571 & 3.286 & 3.571 & 3.571 & 3.714 &  3.429 \\
P($\bar \mu$, $O_0$, $0$)  &               1.905 &   2.571 & 1.857 & 2.000 & 1.714 & 1.714 &  1.571 \\
P($ \mu$, $O_0$, $0$)  &               \textbf{1.310} &   1.143 & 1.286 & 1.429 & 1.286 & 1.286 &  1.429 \\

%  approach &  overall avg. rank \\
%\midrule
%S($\bar \mu$, $O_0$, $0$)  &               3.429 \\
%S($ \mu$, $O_0$, $0$)  &               3.357 \\
%P($\bar \mu$, $O_0$, $0$)  &               1.905 \\
%P($ \mu$, $O_0$, $0$)  &               1.310 \\
\hline
\end{tabular}
%}
\end{table*}

\begin{table*}
\caption{Results for the average rank comparing different labeling of the epidemic.}
\label{tab:pre_process}
\resizebox{\textwidth}{!}{%)
\begin{tabular}{|l|r|r|r|r|r|r|r|}
\hline
approach & overall & $\{\bar T, \bar{S1}, \bar{S2}\}$ &  $\{\bar{T}, S1, \bar{S2}\}$ & $\{\bar{T}, S1, S2\}$ &  $\{ T, \bar{S1}, \bar{S2}\}$ & $\{ T, S1, \bar{S2}\}$ & $\{ T, S1, S2\}$ \\
\hline
\hline
S($\bar \mu$, $O_0$, $0$)  &               6.476 &   6.286 & 5.571 & 4.857 & 7.143 & 7.571 &  7.429 \\
S($\bar \mu$, $O_1$, $0$)  &               6.738 &   7.286 & 6.714 & 6.286 & 6.429 & 7.000 &  6.714 \\
S($\bar \mu$, $O_2$, $0$)  &               5.738 &   6.286 & 5.714 & 5.286 & 5.429 & 6.000 &  5.714 \\
S($\bar \mu$, $O_3$, $0$)  &               \textbf{5.524} &   5.286 & 5.143 & 5.429 & 6.000 & 5.429 &  5.857 \\
P($\bar \mu$, $O_0$, $0$)  &               3.762 &   3.857 & 3.857 & 2.714 & 4.857 & 4.000 &  3.286 \\
P($\bar \mu$, $O_1$, $0$)  &               3.262 &   2.857 & 4.143 & 4.857 & 2.429 & 2.429 &  2.857 \\
P($\bar \mu$, $O_2$, $0$)  &               2.690 &   3.143 & 3.000 & 3.286 & 2.714 & 2.143 &  1.857 \\
P($\bar \mu$, $O_3$, $0$)  &               \textbf{1.810} &   1.000 & 1.857 & 3.286 & 1.000 & 1.429 &  2.286 \\

%approach &  overall avg. rank \\
%\midrule
%S($\bar \mu$, $O_0$, $0$)  &               6.476 \\
%S($\bar \mu$, $O_1$, $0$)  &               6.738 \\
%S($\bar \mu$, $O_2$, $0$)  &               5.738 \\
%S($\bar \mu$, $O_3$, $0$)  &               5.524 \\
%P($\bar \mu$, $O_0$, $0$)  &               3.762 \\
%P($\bar \mu$, $O_1$, $0$)  &               3.262 \\
%P($\bar \mu$, $O_2$, $0$)  &               2.690 \\
%P($\bar \mu$, $O_3$, $0$)  &               1.810 \\
\hline
\end{tabular}

}
\end{table*}

\begin{table*}
\caption{Results of the average rank comparing different window sizes.}
\resizebox{\textwidth}{!}{%)
\label{tab:window}
\begin{tabular}{|l|r|r|r|r|r|r|r|}
\hline
approach & overall & $\{\bar T, \bar{S1}, \bar{S2}\}$ &  $\{\bar{T}, S1, \bar{S2}\}$ & $\{\bar{T}, S1, S2\}$ &  $\{ T, \bar{S1}, \bar{S2}\}$ & $\{ T, S1, \bar{S2}\}$ & $\{ T, S1, S2\}$ \\
\hline
\hline
S($\bar \mu$, $O_0$, $0$)  &              13.381 &  12.143 & 13.286 & 11.286 & 15.571 & 14.429 & 13.571 \\
S($\bar \mu$, $O_0$, $1$)   &              \textbf{12.262} &  12.143 & 10.000 & 12.429 & 10.429 & 12.571 & 16.000 \\
S($\bar \mu$, $O_0$, $2$)   &              14.571 &  14.286 & 14.429 & 14.286 & 14.286 & 13.571 & 16.571 \\
S($\bar \mu$, $O_0$, $3$)   &              15.952 &  16.429 & 15.143 & 16.714 & 15.429 & 16.143 & 15.857 \\
S($\bar \mu$, $O_0$, $4$)   &              15.976 &  16.286 & 16.000 & 16.571 & 15.571 & 17.000 & 14.429 \\
S($\bar \mu$, $O_0$, $5$)   &              15.952 &  16.286 & 17.857 & 14.286 & 16.857 & 16.286 & 14.143 \\
S($\bar \mu$, $O_0$, $6$)   &              16.024 &  17.000 & 16.857 & 14.143 & 16.286 & 16.143 & 15.714 \\
S($\bar \mu$, $O_0$, $7$)   &              15.310 &  15.571 & 16.571 & 15.000 & 14.429 & 15.429 & 14.857 \\
S($\bar \mu$, $O_0$, $8$)   &              16.429 &  16.000 & 16.143 & 16.857 & 15.857 & 16.571 & 17.143 \\
S($\bar \mu$, $O_0$, $9$)   &              16.762 &  17.000 & 16.429 & 18.571 & 16.000 & 16.857 & 15.714 \\
P($\bar \mu$, $O_0$, $0$)  &               6.929 &   7.714 &  7.000 &  8.000 &  6.143 &  4.857 &  7.857 \\
P($\bar \mu$, $O_0$, $1$)  &               \textbf{4.619} &   4.571 &  3.286 &  6.429 &  4.286 &  5.714 &  3.429 \\
P($\bar \mu$, $O_0$, $2$)  &               5.905 &   6.857 &  6.143 &  5.429 &  5.857 &  6.000 &  5.143 \\
P($\bar \mu$, $O_0$, $3$)  &               6.286 &   5.429 &  7.286 &  6.714 &  6.714 &  7.714 &  3.857 \\
P($\bar \mu$, $O_0$, $4$)  &               6.429 &   5.857 &  6.857 &  5.714 &  7.143 &  6.857 &  6.143 \\
P($\bar \mu$, $O_0$, $5$)  &               6.048 &   5.857 &  6.143 &  4.714 &  6.857 &  6.286 &  6.429 \\
P($\bar \mu$, $O_0$, $6$)  &               5.714 &   6.286 &  5.286 &  5.286 &  5.571 &  5.143 &  6.714 \\
P($\bar \mu$, $O_0$, $7$)  &               5.262 &   6.286 &  4.857 &  5.571 &  4.143 &  4.714 &  6.000 \\
P($\bar \mu$, $O_0$, $8$)  &               5.190 &   3.714 &  5.571 &  5.714 &  6.714 &  4.714 &  4.714 \\
P($\bar \mu$, $O_0$, $9$)  &               5.000 &   4.286 &  4.857 &  6.286 &  5.857 &  3.000 &  5.714 \\
%approach &  overall avg. rank \\
%\midrule
%S($\bar \mu$, $O_0$, $0$)  &              13.381  \\
%S($\bar \mu$, $O_0$, $1$)  &              12.262  \\
%S($\bar \mu$, $O_0$, $2$)  &              14.571  \\
%S($\bar \mu$, $O_0$, $3$)  &              15.952  \\
%S($\bar \mu$, $O_0$, $4$)  &              15.976  \\
%S($\bar \mu$, $O_0$, $5$)  &              15.952  \\
%S($\bar \mu$, $O_0$, $6$)  &              16.024  \\
%S($\bar \mu$, $O_0$, $7$)  &              15.310  \\
%S($\bar \mu$, $O_0$, $8$)  &              16.429  \\
%S($\bar \mu$, $O_0$, $9$)  &              16.762  \\
%P($\bar \mu$, $O_0$, $0$)  &               6.929  \\
%P($\bar \mu$, $O_0$, $1$) &               4.619  \\
%P($\bar \mu$, $O_0$, $2$)  &               5.905  \\
%P($\bar \mu$, $O_0$, $3$)  &               6.286  \\
%P($\bar \mu$, $O_0$, $4$)  &               6.429  \\
%P($\bar \mu$, $O_0$, $5$)  &               6.048  \\
%P($\bar \mu$, $O_0$, $6$)  &               5.714  \\
%P($\bar \mu$, $O_0$, $7$)  &               5.262 \\
%P($\bar \mu$, $O_0$, $8$)  &               5.190  \\
%P($\bar \mu$, $O_0$, $9$)  &               5.000  \\
\hline
\end{tabular}

}
\end{table*}

\begin{table*}
\caption{Results for  the average rank for including the average in the dataset.}
%\scriptsize
%\resizebox{\textwidth}{!}{%)
\begin{tabular}{rrrrrc}
\toprule
$\text{average}_{t}$ & $\text{RKI}_{t-1}$ & $\text{RKI}_{t}$ & $\text{Bayes}_{t-1}$ & $\text{Bayes}_{t}$ & $\text{outbreak}_{t}$\\
\midrule
\dots & \dots & \ldots & \dots & \dots & \ldots\\
1.00 & 0.59 & 0.86 & 0.63 & 0.63 & no\\
0.50 & 0.86 & 0.26 & 0.63 & 0.14 & no\\
0.50 & 0.26 & 0.63 & 0.14 & 0.43 & no\\
0.50 & 0.63 & 0.00 & 0.43 & 0.00 & yes\\
1.50 & 0.00 & 0.14 & 0.00 & 0.10 & yes\\
2.25 & 0.14 & 0.00 & 0.10 & 0.00 & yes\\
4.50 & 0.00 & 0.13 & 0.00 & 0.12 & yes\\
6.25 & 0.13 & 0.83 & 0.12 & 0.73 & yes\\
6.00 & 0.83 & 0.99 & 0.73 & 0.98 & yes\\
5.50 & 0.99 & 1.00 & 0.98 & 0.99 & no\\
\dots & \dots & \ldots & \dots & \dots & \ldots\\
\bottomrule
\end{tabular}
%}
\end{table*}

\begin{figure*}[t!]
\centering
\includegraphics[width=1\textwidth]{figures/dataset_creation.pdf}
\label{figure:DRandTPR}
\end{figure*}

\begin{table*}
\caption{Results for  the average rank for including the average in the dataset.}
%\scriptsize
%\resizebox{\textwidth}{!}{%)
\begin{tabular}{rrrrrc}
\toprule
$\text{average}_{t}$ & $\text{RKI}_{t-1}$ & $\text{RKI}_{t}$ & $\text{Bayes}_{t-1}$ & $\text{Bayes}_{t}$ & $\text{outbreak}_{t}$\\
\midrule
\dots & \dots & \ldots & \dots & \dots & \ldots\\
1.00 & 0.59 & 0.86 & 0.63 & 0.63 & no\\
0.50 & 0.86 & 0.26 & 0.63 & 0.14 & no\\
0.50 & 0.26 & 0.63 & 0.14 & 0.43 & no\\
0.50 & 0.63 & 0.00 & 0.43 & 0.00 & yes\\
1.50 & 0.00 & 0.14 & 0.00 & 0.10 & yes\\
2.25 & 0.14 & 0.00 & 0.10 & 0.00 & yes\\
4.50 & 0.00 & 0.13 & 0.00 & 0.12 & yes\\
6.25 & 0.13 & 0.83 & 0.12 & 0.73 & yes\\
6.00 & 0.83 & 0.99 & 0.73 & 0.98 & yes\\
5.50 & 0.99 & 1.00 & 0.98 & 0.99 & no\\
\dots & \dots & \ldots & \dots & \dots & \ldots\\
\bottomrule
\end{tabular}
%}
\end{table*}

\begin{tabular}{l|c|r}
  \hline
  Some & \cellcolor{blue!25}coloured & contents \\
  \hline
\end{tabular}

\begin{table*}
\caption{Comparison of different window sizes for the data (including the average and using the labeling $O_0$).%:  \emph{overall} denotes all 42 test cases, $\{(\neg)T, (\neg)S1, (\neg)S2\}$ only cases (not) containing trend, annual/biannual seasonality, respectively.
}
%\resizebox{\textwidth}{!}{%)
%\large
\label{tab:window_1_2_4_8_12}
\begin{tabular}{lrrrrrrr}
\toprule
Approach & Overall & $\{\neg{T}, \neg{S1}, \neg{S2}\}$ &  $\{\neg{T}, S1, \neg{S2}\}$ & $\{\neg{T}, S1, S2\}$ &  $\{ T, \neg{S1}, \neg{S2}\}$ & $\{ T, S1, \neg{S2}\}$ & $\{ T, S1, S2\}$ \\
\midrule
    S($\neg \mu$,$O_0$, &               8.524 &   8.143 &  8.429 &  7.143 &  9.571 &  9.286 &  8.571 \\
  S($\neg \mu$,$O_0$,1) &               7.571 &   7.857 &  6.143 &  7.714 &  6.429 &  7.714 &  9.571 \\
  S($\neg \mu$,$O_0$,2) &               9.476 &   9.429 &  9.714 &  9.286 &  9.429 &  9.000 & 10.000 \\
  S($\neg \mu$,$O_0$,4) &               9.905 &  10.286 & 10.429 &  9.857 &  9.571 & 10.429 &  8.857 \\
  S($\neg \mu$,$O_0$,8) &              10.000 &   9.857 & 10.143 & 10.143 &  9.429 & 10.429 & 10.000 \\
  S($\neg \mu$,$O_0$,12) &              10.405 &  10.571 & 10.571 & 11.143 & 10.286 & 10.143 &  9.714 \\
  \midrule
    P($\neg \mu$,$O_0$, &               4.405 &   5.143 &  4.429 &  5.000 &  3.857 &  3.286 &  4.714 \\
  P($\neg \mu$,$O_0$,1) &               3.000 &   2.714 &  2.286 &  3.857 &  2.857 &  3.714 &  2.571 \\
  P($\neg \mu$,$O_0$,2) &               3.857 &   4.429 &  4.286 &  3.429 &  4.000 &  3.857 &  3.143 \\
  P($\neg \mu$,$O_0$,4) &               4.119 &   3.714 &  4.429 &  3.429 &  4.429 &  4.571 &  4.143 \\
  P($\neg \mu$,$O_0$,8) &               3.476 &   2.714 &  3.429 &  4.143 &  4.143 &  3.429 &  3.000 \\

 P($\neg \mu$,$O_0$,12) &               3.262 &   3.143 &  3.714 &  2.857 &  4.000 &  2.143 &  3.714 \\
\bottomrule
\end{tabular}

\end{table*}

\begin{table*}
\caption{Comparison of different window sizes for the data (including the average and using the labeling $O_0$).%:  \emph{overall} denotes all 42 test cases, $\{(\neg)T, (\neg)S1, (\neg)S2\}$ only cases (not) containing trend, annual/biannual seasonality, respectively.
}
%\resizebox{\textwidth}{!}{%)
%\large
\label{tab:old10____window}
\begin{tabular}{lrrrrrrr}
\toprule
Approach & Overall & $\{\neg{T}, \neg{S1}, \neg{S2}\}$ &  $\{\neg{T}, S1, \neg{S2}\}$ & $\{\neg{T}, S1, S2\}$ &  $\{ T, \neg{S1}, \neg{S2}\}$ & $\{ T, S1, \neg{S2}\}$ & $\{ T, S1, S2\}$ \\
\midrule
S($\neg \mu$, $O_0$, $0$)  &              13.381 &  12.143 & 13.286 & 11.286 & 15.571 & 14.429 & 13.571 \\
S($\neg \mu$, $O_0$, $1$)   &              \textbf{12.262} &  12.143 & 10.000 & 12.429 & 10.429 & 12.571 & 16.000 \\
S($\neg \mu$, $O_0$, $2$)   &              14.571 &  14.286 & 14.429 & 14.286 & 14.286 & 13.571 & 16.571 \\
S($\neg \mu$, $O_0$, $3$)   &              15.952 &  16.429 & 15.143 & 16.714 & 15.429 & 16.143 & 15.857 \\
S($\neg \mu$, $O_0$, $4$)   &              15.976 &  16.286 & 16.000 & 16.571 & 15.571 & 17.000 & 14.429 \\
\midrule
S($\neg \mu$, $O_0$, $5$)   &              15.952 &  16.286 & 17.857 & 14.286 & 16.857 & 16.286 & 14.143 \\
S($\neg \mu$, $O_0$, $6$)   &              16.024 &  17.000 & 16.857 & 14.143 & 16.286 & 16.143 & 15.714 \\
S($\neg \mu$, $O_0$, $7$)   &              15.310 &  15.571 & 16.571 & 15.000 & 14.429 & 15.429 & 14.857 \\
S($\neg \mu$, $O_0$, $8$)   &              16.429 &  16.000 & 16.143 & 16.857 & 15.857 & 16.571 & 17.143 \\
S($\neg \mu$, $O_0$, $9$)   &              16.762 &  17.000 & 16.429 & 18.571 & 16.000 & 16.857 & 15.714 \\
\midrule
P($\neg \mu$, $O_0$, $0$)  &               6.929 &   7.714 &  7.000 &  8.000 &  6.143 &  4.857 &  7.857 \\
P($\neg \mu$, $O_0$, $1$)  &               \textbf{4.619} &   4.571 &  3.286 &  6.429 &  4.286 &  5.714 &  3.429 \\
P($\neg \mu$, $O_0$, $2$)  &               5.905 &   6.857 &  6.143 &  5.429 &  5.857 &  6.000 &  5.143 \\
P($\neg \mu$, $O_0$, $3$)  &               6.286 &   5.429 &  7.286 &  6.714 &  6.714 &  7.714 &  3.857 \\
P($\neg \mu$, $O_0$, $4$)  &               6.429 &   5.857 &  6.857 &  5.714 &  7.143 &  6.857 &  6.143 \\
\midrule
P($\neg \mu$, $O_0$, $5$)  &               6.048 &   5.857 &  6.143 &  4.714 &  6.857 &  6.286 &  6.429 \\
P($\neg \mu$, $O_0$, $6$)  &               5.714 &   6.286 &  5.286 &  5.286 &  5.571 &  5.143 &  6.714 \\
P($\neg \mu$, $O_0$, $7$)  &               5.262 &   6.286 &  4.857 &  5.571 &  4.143 &  4.714 &  6.000 \\
P($\neg \mu$, $O_0$, $8$)  &               5.190 &   3.714 &  5.571 &  5.714 &  6.714 &  4.714 &  4.714 \\
P($\neg \mu$, $O_0$, $9$)  &               5.000 &   4.286 &  4.857 &  6.286 &  5.857 &  3.000 &  5.714 \\
\bottomrule
\end{tabular}

\end{table*}

\begin{table*}
\caption{Comparison of different window sizes for the data (including the average and using the labeling $O_0$).%:  \emph{overall} denotes all 42 test cases, $\{(\neg)T, (\neg)S1, (\neg)S2\}$ only cases (not) containing trend, annual/biannual seasonality, respectively.
}
%\resizebox{\textwidth}{!}{%)
%\large
\label{tab:window12____old}
\begin{tabular}{lrrrrrrr}
\toprule
Approach & Overall & $\{\neg{T}, \neg{S1}, \neg{S2}\}$ &  $\{\neg{T}, S1, \neg{S2}\}$ & $\{\neg{T}, S1, S2\}$ &  $\{ T, \neg{S1}, \neg{S2}\}$ & $\{ T, S1, \neg{S2}\}$ & $\{ T, S1, S2\}$ \\
\midrule
    S($\neg \mu$,$O_0$, 0)&              17.048 &  15.857 & 16.714 & 13.857 & 20.143 & 18.429 & 17.286 \\
  S($\neg \mu$,$O_0$, 1) &              \textbf{15.524} &  15.571 & 12.714 & 15.429 & 13.429 & 16.000 & 20.000 \\
  S($\neg \mu$,$O_0$, 2) &              18.524 &  18.286 & 18.429 & 18.143 & 18.000 & 17.143 & 21.143 \\
  S($\neg \mu$,$O_0$, 3) &              20.071 &  20.571 & 19.000 & 20.714 & 19.429 & 20.714 & 20.000 \\
  S($\neg \mu$,$O_0$, 4) &              19.929 &  20.286 & 20.000 & 20.286 & 19.286 & 21.286 & 18.429 \\
  S($\neg \mu$,$O_0$, 5) &              20.190 &  20.286 & 22.143 & 17.714 & 21.714 & 20.857 & 18.429 \\
  \midrule
  S($\neg \mu$,$O_0$, 6) &              20.310 &  21.571 & 21.000 & 17.429 & 21.000 & 20.429 & 20.429 \\
  S($\neg \mu$,$O_0$, 7) &              19.214 &  19.429 & 20.714 & 18.857 & 18.000 & 19.143 & 19.143 \\
  S($\neg \mu$,$O_0$, 8) &              20.595 &  20.000 & 19.571 & 21.143 & 19.857 & 21.000 & 22.000 \\
  S($\neg \mu$,$O_0$, 9) &              20.786 &  20.857 & 19.857 & 22.857 & 19.857 & 21.143 & 20.143 \\
  S($\neg \mu$,$O_0$, 10) &              20.833 &  19.286 & 22.429 & 20.000 & 19.714 & 22.571 & 21.000 \\
 S($\neg \mu$,$O_0$, 11) &              21.857 &  23.000 & 22.714 & 22.429 & 20.857 & 20.857 & 21.286 \\
 S($\neg \mu$,$O_0$, 12) &              21.690 &  22.714 & 22.000 & 23.714 & 21.714 & 20.429 & 19.571 \\
\midrule
P($\neg \mu$,$O_0$, 0)&               8.833 &  10.143 &  8.857 & 10.000 &  7.571 &  6.714 &  9.714 \\
  P($\neg \mu$,$O_0$, 1) &               \textbf{5.952} &   6.000 &  4.143 &  8.429 &  5.143 &  7.429 &  4.571 \\
  P($\neg \mu$,$O_0$, 2) &               7.714 &   8.857 &  8.286 &  7.286 &  7.286 &  8.143 &  6.429 \\
  P($\neg \mu$,$O_0$, 3) &               8.119 &   7.429 &  9.143 &  8.714 &  8.429 & 10.143 &  4.857 \\
  P($\neg \mu$,$O_0$, 4) &               8.357 &   7.714 &  8.571 &  7.714 &  9.286 &  9.286 &  7.571 \\
  P($\neg \mu$,$O_0$, 5) &               7.952 &   7.857 &  8.143 &  6.429 &  8.571 &  8.714 &  8.000 \\
  \midrule
  P($\neg \mu$,$O_0$, 6) &               7.643 &   8.714 &  7.286 &  7.429 &  7.000 &  7.286 &  8.143 \\
  P($\neg \mu$,$O_0$, 7) &               6.857 &   8.286 &  6.000 &  7.571 &  4.714 &  6.571 &  8.000 \\
  P($\neg \mu$,$O_0$, 8) &               6.810 &   4.857 &  6.571 &  8.000 &  8.857 &  6.857 &  5.714 \\
  P($\neg \mu$,$O_0$, 9) &               6.548 &   6.000 &  6.286 &  8.714 &  7.000 &  4.286 &  7.000 \\
 P($\neg \mu$,$O_0$, 10) &               6.310 &   6.429 &  6.714 &  7.714 &  6.000 &  3.571 &  7.429 \\
 P($\neg \mu$,$O_0$, 11) &               7.048 &   5.714 &  6.857 &  5.000 &  9.714 &  7.143 &  7.857 \\
 P($\neg \mu$,$O_0$, 12) &               6.286 &   5.286 &  6.857 &  5.429 &  8.429 &  4.857 &  6.857 \\
\bottomrule
\end{tabular}

\end{table*}

\begin{figure*}
    \begin{minipage}{0.45\linewidth}
		\centering
		\includegraphics[width=\linewidth]{figures/ts.pdf}
	\end{minipage}\hfill
	\begin{minipage}{0.5\linewidth}
		\centering
		\begin{tabular}{rrrrrc}
\toprule
$\text{average}_{t}$ & $\text{RKI}_{t-1}$ & $\text{RKI}_{t}$ & $\text{Bayes}_{t-1}$ & $\text{Bayes}_{t}$ & $\text{outbreak}_{t}$\\
\midrule
\dots & \dots & \ldots & \dots & \dots & \ldots\\
1.00 & 0.59 & 0.86 & 0.63 & 0.63 & no\\
0.50 & 0.86 & 0.26 & 0.63 & 0.14 & no\\
0.50 & 0.26 & 0.63 & 0.14 & 0.43 & no\\
0.50 & 0.63 & 0.00 & 0.43 & 0.00 & yes\\
1.50 & 0.00 & 0.14 & 0.00 & 0.10 & yes\\
2.25 & 0.14 & 0.00 & 0.10 & 0.00 & yes\\
4.50 & 0.00 & 0.13 & 0.00 & 0.12 & yes\\
6.25 & 0.13 & 0.83 & 0.12 & 0.73 & yes\\
6.00 & 0.83 & 0.99 & 0.73 & 0.98 & yes\\
5.50 & 0.99 & 1.00 & 0.98 & 0.99 & no\\
\dots & \dots & \ldots & \dots & \dots & \ldots\\
\bottomrule
\end{tabular}
	\end{minipage}
\captionof{figure}{2-D scatterplot of the Student Database}
\end{figure*}

\begin{figure*}[t!]
%left
\includegraphics[width=1.\textwidth]{figures/dataset_creation_long_table2.pdf}
\caption{Example for the creation of training data for the learning algorithm including  the statistical algorithms Bayes and RKI and the mean over the previous four counts ($m=4$) as features and a window size of one ($w=1$). On the left hand side, the time series for a particular disease is visualized representing the number of cases of infections over time. Underneath the computed $p$-values of the statistical algorithms and the label indicating an outbreak for each observation are placed at the respective time index. Using this information the data instances can be created as shown on the right. Each particular time point is represented by one training. The colorized frames help to indicate the respective values.
%The table on the right hand side represents the created data for the ML approach which is constructed with the information of the time series, the labeling of the outbreak and the $p$-values of the statistical methods on the left hand side.
}
\label{figure:example_dataset_creation}
\end{figure*}
